# Supplementary material for: Beyond Detection: Governing GenAI in Academic Peer Review as a Sociotechnical Challenge
Source: arXiv:2603.20214 source file (2026-03-02)
Supplement: Supplementary file 1 [file appendix.tex]

\appendix

\section{Participant Recruitment}
